# Supplementary material for: A StrongREJECT for Empty Jailbreaks
Source: arXiv:2402.10260 source file (2024-08-27)
Supplement: Supplementary file 3 [file jailbreak_scores_by_category.tex]

\section{Jailbreak Scores by Category}
In \cref{fig:jailbreak_by_category}, we can see that jailbreak scores vary in effectiveness by category. This plot shows average jailbreak scores across the 50-question StrongREJECT-small subset scored by both humans and models (with Dolphin excluded). We see that the Disinformation and deception category is easiest to jailbreak, suggesting that researchers should focus especially on misuse risk in this area (for instance, the possibility of automating propaganda or scams).

\begin{figure}[H]
	\centering
	\begin{subfigure}[b]{.65\textwidth}
    	\includegraphics{figures/human_score_by_category2.pdf}
    	\caption{Jailbreak scores per category, scored by humans.}
    	\label{fig:jailbreak_by_category_humans}
	\end{subfigure}
	\hfill \\
        \begin{subfigure}[b]{0.65\textwidth}
    	\includegraphics{figures/model_score_by_category1.pdf}
    	\caption{Jailbreak scores per category, scored by StrongREJECT GPT-4.}
    	\label{fig:jailbreak_by_category_ours}
	\end{subfigure}
        \hfill \\
	\begin{subfigure}[b]{0.65\textwidth}
    	\includegraphics{figures/model_score_by_category2.pdf}
    	\caption{Jailbreak scores per category, scored by StrongREJECT fine-tuned.}
    	\label{fig:jailbreak_by_category_ours}
	\end{subfigure}
    
	\caption{Jailbreak scores per category}
	\label{fig:jailbreak_by_category}
\end{figure}

\clearpage
